# Supplementary material for: SAUC: Sparsity-Aware Uncertainty Calibration for Spatiotemporal Prediction with Graph Neural Networks
Source: arXiv:2409.08766 source file (2024-09-13)
Supplement: Supplementary file 1 [file Appendix.tex]

\clearpage
\section{Appendix}

\subsection{Motivations (notes)}
\redfont{The negative binomial distributions easily variance of the dispersion. This is ridiculous. The value will be very large if we did not clip, say set the maximum values of, the expected outputs. Suce dispersion makes it hard to capture the variance of the discrete data. Especially we are looking for the error-based calibration errors.}

\subsection{Reproducibility}

\subsection{Implementation of Probabilistic STDL}
Introduce how we reformat the numerical-output spatiotemporal neural networks into the mean-variance prediction one.

\redfont{Show the performance of modified Negative Binomial prediction v.s. the original one}.

\redfont{Not necessarily need to put them into the context or include all the metrics in the main content.}

\begin{table*}[htbp]
    \centering
    \begin{tabular}{cc|ccc}
    \toprule
        Dataset & Models & MAE & MSE & RMSE \\        
    \midrule
        \multirow{2}{*}{CCR\_1h} & STGCN & 0.429 &    0.406 &   0.637 \\
                     & STGCN-NB & 0.317 &    0.494 &   0.703 \\
                     & GWN  & 0.848 &    0.926 &   0.962 \\
                     & GWN-NB  & 0.334 &    0.587 &   0.766 \\
        \hdashline
        
        \multirow{2}{*}{CCR\_8h} & STGCN & 1.499 &    5.691 &   2.386 \\
                                   & STGCN-NB& 1.452 &    5.413 &   2.326 \\
                     & GWN  & 1.395 &    4.212 &   2.052 \\
                     & GWN-NB  & 1.478 &   5.645 &   2.376 \\
        \hdashline
        
        \multirow{2}{*}{CCR\_daily} & STGCN & 2.951 &   26.698 &   5.167 \\
                     & STGCN-NB & 2.719 &   18.368 &   4.286 \\
                     & GWN  & 2.521 &   14.316 &   3.784 \\
                     & GWN-NB  & 2.681 &   19.152 &   9.703 \\
        \hdashline 
        
        \multirow{2}{*}{CCR\_weekly} & STGCN & 14.146 &  544.415 &  23.333 \\
                     & STGCN-NB & 12.505 &  409.741 &  20.242 \\
                     & GWN  & 9.938 &  259.311 &  16.103 \\
                     & GWN-NB  & 14.516 &  539.679 &  23.231 \\
        
    \hline
        \multirow{2}{*}{CTC\_1h} & STGCN & 0.084 &   0.046 &  0.214 \\
        & STGCN-NB & 0.044 &    0.048 &    0.220 \\
                    & GWN  & 0.960 &    0.960 &   0.980 \\
                    & GWN-NB  & 0.044 &  0.048 &   0.220 \\
        \hdashline
        
        \multirow{2}{*}{CTC\_8h} & STGCN & 0.453 &   0.401 &  0.633 \\
        & STGCN-NB & 0.346 &    0.527 &   0.726 \\
                    & GWN  & 0.810 &   0.855 &  0.924 \\
                    & GWN-NB  & 0.352 &  0.557 &  0.746 \\
        \hdashline
        
        \multirow{2}{*}{CTC\_daily} & STGCN & 0.861 &   1.318 &  1.148 \\
        & STGCN-NB & 1.433 &  3.193 &  1.786 \\
                & GWN  & 0.895 &   1.332 &  1.154 \\
                & GWN-NB  & 1.019 &  2.404 &   1.55 \\
        \hdashline
        
        \multirow{2}{*}{CTC\_weekly} & STGCN & 2.474 &  11.004 &  3.317 \\ 
        & STGCN-NB & 3.618 &   15.442 &   3.929 \\
        & GWN  & 2.423 &  10.098 &  3.178 \\
        & GWN-NB & 3.279 &  13.608 &  3.689 \\
    \bottomrule
    \end{tabular}
    \caption{Comparisons between modified models and the original models.}
    \label{tab:appendix_modification}
\end{table*}

    % \hline
        
    %     \multirow{2}{*}{SLD\_5min} & STGCN  &   0.198 &  0.165 &  0.406 \\
    %     & STGCN-NB & 0.153 &  0.238 &  0.488 \\
    %     & GWN  & & & \\
    %     & GWN-NB  & & & \\
        
    %     \hdashline
    %     \multirow{2}{*}{SLD\_15min} & STGCN  &   0.409 &  0.548 &  0.741 \\
    %     & STGCN-NB & 0.374 &  0.825 &  0.908 \\
    %     & GWN  & & & \\
    %     & GWN-NB  & & & \\
    %     \hdashline


    %     \multirow{2}{*}{SLD\_60min} & STGCN  &   0.953 &  3.127 &  1.768 \\
    %     & STGCN-NB & 1.213 &  6.329 &  2.516 \\
    %     & GWN  & & & \\
    %      & GWN-NB  & & & \\


Our modification modifies the last layer. When the output layer of the model is about to output the numerical value outputs, we change the output layer into mean and variance prediction instead.

In addition, we change the loss function from the MSE Loss or MAE Loss into Cross Entropy Loss. As shown in Table \ref{tab:appendix_modification}, the error terms are a little bit smaller than the original model. 

\subsection{Data Description and sparsity discussion}
We incorporate different sources of spatiotemporal datasets. 
\subsubsection{Data Descriptions}
\begin{enumerate}[label=(\arabic*)]
    \item Chicago Traffic Crash (CTC)\footnote{\url{https://data.cityofchicago.org/Transportation/Traffic-Crashes-Crashes/85ca-t3if}} collected from 277 police beats from Jan 1, 2016 to Jan 1, 2023; 
    \item Chicago Crime Records (CCR)\footnote{\url{https://data.cityofchicago.org/Public-Safety/Crimes-2001-to-Present/ijzp-q8t2}} collected from 77 census tracts from Jan 1, 2003 to Jan 1, 2023
    \item Smart Location Database (SLD)\footnote{\url{https://www1.nyc.gov/site/tlc/about/tlc-trip-record-data.page}} records For-Hire Vehicle (FHV) trip records in the Manhattan area (divided into 67 zones by administrative zip codes) from January 2018 to April 2018.
\end{enumerate}

In the spatiotemporal dataset, the granularity of the temporal resolutions will result in different levels of resolutions, which are important. 

For crime and accident data, we control the data sparsity by varying the temporal resolution. We vary the temporal resolution from weekly, daily, 8 hours, and 1 hour. Such division is based on the fact that crime and accident data less frequently happened on the city scale. 

For sparse travel demand data, we also aggregate and divide the data into 60min, 15min, and 5min. This is the same setting in \citep{zhuang2022uncertainty,jiang2023uncertainty}. The travel demand resolutions are divided into minutes because they need more granular prediction results for swifter responses. Previous spatiotemporal deep learning literature frequently uses these resolutions. Specific data statistics can be found in Table \ref{tab:data_sparsity}. The sparsity means the portion of zeroes in the data entries.


\begin{figure*}[htbp]
    \centering
    \subfigure[Kernel density estimate (KDE) plot]{\includegraphics[width=0.45\linewidth]{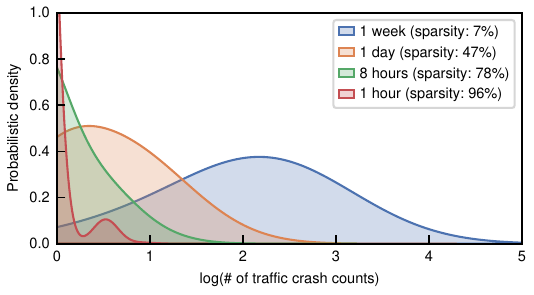}}\hfill
    \subfigure[Cumulative density function (CDF) plot]{\includegraphics[width=0.45\linewidth]{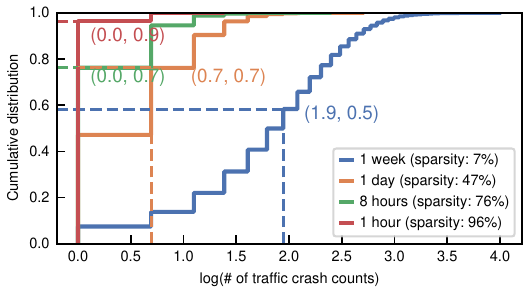}}
    
    \caption{Comparative visualization of log-transformed crime counts for different temporal resolutions in the Chicago traffic crash dataset: (a) The KDE plot demonstrates the asymmetric data distribution shape in fine resolutions. (b) The CDF plot illustrates emphasizing the asymmetry. Median values are marked by vertical dashed lines, and horizontal lines quantify the data below the median, where a value of 0.5 denotes symmetry. 'Sparsity' denotes the proportion of zero-count instances within each temporal resolution.}
    \label{fig:sparsity_transition}
\end{figure*}
\redfont{Describe the plot accordingly}

\subsubsection{Spatial Distributions}
Add spatial distributions of datasets. How does the results look like from the map.

\subsubsection{Adjacency Matrix}

The construction of the adjacency matrix is more based on geographical distances. For
crash and crime data, we calculate the distances of centroids between different regions. 

\subsubsection{Negative Binomial Distributions}
\redfont{We need some histograms and fitted figures that could show that our data can reflect the negative binomial distributions.} This is important.

\subsubsection{Sparsity Patterns}
\redfont{To compare the results, we compare the reliability diagram and spatial distributions of the residuals. We want to show some aggregated spatial pattern to demonstrate why it is important to include the spatial modules and why calibration is important.}

% \begin{table}[htbp]
%     \centering
%     \begin{tabular}{c|cc}
%     \toprule
%         Dataset & ECE & ECE for Calibrated \\        
%     \midrule
%         Crash\_1h & / & 0.050 \\
%         Crash\_8h & 0.175 & 0.035 \\
%         Crash\_daily & 0.501 & $<0.001$\\
%         Crash\_weekly & 0.564 & 0.122\\
%     \hline
%         Crime\_1h & 0.255 & 0.062\\
%         Crime\_8h & 0.367 & 0.052\\
%         Crime\_daily & 0.427 & 0.186 \\
%         Crime\_weekly & / & $<0.001$\\
%     \bottomrule
%     \end{tabular}
%     \caption{Calibration error comparisons for Softmax modified outputs. The calibration is built using isotonic regression. This table aims to clarify the importance of calibration errors in sparse data.}
%     \label{tab:softmax_ece_tables}
% \end{table}

% \begin{table}[htbp]
%     \centering
%     \begin{tabular}{c|ccccc}
%     \toprule
%         Dataset & UCE & ENCE & PICP & MPIW & PMCE \\        
%     \midrule
%         Crash\_1h &  &  &  &  &\\
%         Crash\_8h &  &  &  &  &\\
%         Crash\_daily &  &  &  &  &\\
%         Crash\_weekly &  &  &  &  &\\
%     \hline
%         Crime\_1h &  &  &  &  & \\
%         Crime\_8h &  &  &  &  & \\
%         Crime\_daily &  &  &  &  &\\
%         Crime\_weekly &  &  &  &  &\\
%     \bottomrule
%     \end{tabular}
%     \caption{Calibration error comparisons for Negative Binomial modified outputs before they get calibrated.}
%     \label{tab:nb_ce_tables}
% \end{table}

\subsection{Residuals Contains Spatiotemporal Patterns}
Do we need to include the residual distributions? \redfont{We could show whether the calibration error has the spatial patterns like the residuals. We could include both.}

\subsection{Calibration Errors}
There are various calibration errors. The calibration errors are initially proposed to deal with the binary classification problems. The 

% \begin{table*}[htbp]
%     \scriptsize
%     \centering
%     \begin{tabular}{lrrrrrrrrrrrr}
%     \toprule
%     {} & \multicolumn{6}{l}{UCE} & \multicolumn{6}{l}{ENCE} \\
%     method & before\_calib & histogram & isotonic & our\_calib &   platt & temperature & before\_calib & histogram & isotonic & our\_calib &  platt & temperature \\
%     interval &              &           &          &           &         &             &              &           &          &           &        &             \\
%     \midrule
%     CTC\_1h       &        0.160 &     0.222 &    0.227 &     0.403 &   0.179 &       0.153 &         0.082 &     0.214 &    0.210 &     0.028 &  0.163 &       0.114 \\
%     CTC\_8h       &        3.468 &     1.210 &    1.082 &     0.623 &   0.757 &       2.258 &        0.189 &     0.200 &    0.136 &     0.040 &  0.079 &       0.211 \\
%     CTC\_daily    &        0.011 &     9.117 &    8.845 &     0.373 &   9.101 &       2.475 &        0.003 &     0.075 &    0.060 &     0.265 &  0.079 &       0.422 \\
%     CTC\_1w       &       40.182 &     4.857 &    9.745 &     4.297&  44.003 &      31.624 &        1.482 &     0.850 &    1.048 &     0.225 &  1.596 &       0.833 \\
%     \bottomrule
%     \toprule
%     CCR\_1h       &        1.526 &     2.386 &    4.418 &     3.181 &     2.187 &       1.452 &        0.217 &     0.199 &    0.160 &     0.207 &  0.185 &       0.215 \\
%     CCR\_8h       &       28.916 &    10.239 &    7.337 &    11.394 &     3.851 &       7.099 &        0.315 &     0.097 &    0.048 &     0.190 &  0.210 &       0.241 \\
%     CCR\_daily    &       81.517 &    53.569 &   38.674 &   50.769 &   53.142 &      65.152 &        0.505 &     0.238 &    0.185 &     0.275 &  0.873 &       0.468 \\
%     CCR\_1w       &      593.065 &   677.845 &  458.748 &  224.740 &  326.511 &     461.005 &        0.415 &     0.403 &     0.414&     0.342 &  1.965 &       0.416 \\
        
%     \bottomrule
    
%     \bottomrule
%     \end{tabular}
%     \caption{Calibration errors of full observations}
%     \label{tab:ce_full_appendix}
% \end{table*}

% \begin{table*}[htbp]
%     \scriptsize
%     \centering    
    
%     \begin{tabular}{lrrrrrrrrrrrr}
%     \toprule
%     {} & \multicolumn{6}{l}{UCE} & \multicolumn{6}{l}{ENCE} \\
%     method & before\_calib & histogram & isotonic & our\_calib &  platt & temperature & before\_calib & histogram & isotonic & our\_calib &  platt & temperature \\
%     interval    &              &           &          &           &        &             &              &           &          &           &        &             \\
%     \midrule
%     CTC\_1h       &        0.156 &     0.238 &    0.223 &     0.000 &  0.257 &       0.114 &        0.042 &     0.702 &    0.579 &     0.000 &  0.596 &       0.381 \\
%     CTC\_8h       &        3.276 &     0.853 &    0.618 &     0.000 &  0.564 &       2.256 &        0.213 &     0.226 &    0.131 &     0.000 &  0.168 &       0.255 \\
%     CTC\_daily    &        0.001 &     3.801 &    2.848 &     0.000 &  4.062 &       1.163 &        0.007 &     0.154 &    0.078 &     0.000 &  0.240 &       0.537 \\
%     CTC\_1w       &       13.220 &    26.212 &   18.689 &    12.259 &  9.756 &      19.431 &        0.814 &     1.447 &    1.237 &     0.196 &  0.958 &       0.754 \\
%     \bottomrule
%     \toprule
%     CCR\_1h       &        5.436 &     0.777 &    0.592 &     0.000 &  1.011 &       3.345 &        0.524 &     0.189 &    0.129 &     0.000 &  0.362 &       0.500 \\
%     CCR\_8h       &       23.318 &     4.970 &    8.748 &     6.829 &  0.540 &       9.761 &        0.208 &     0.159 &    0.226 &     0.052 &  0.062 &       0.303 \\
%     CCR\_daily    &       30.930 &    20.696 &   20.357 &    18.978 &  3.482 &      23.036 &        0.991 &     0.977 &    0.732 &     0.284 &  0.208 &       0.868 \\
%     CCR\_1w       &        1.886 &    57.233 &    2.112 &     3.164 &  2.260 &       1.418 &        0.145 &     1.084 &    0.143 &     0.058 &  0.151 &       0.108 \\
%     \bottomrule
%     \bottomrule
%     \end{tabular}
%     \caption{Calibration errors of observation values are zeores.}
%     \label{tab:ce_zero_appendix}
% \end{table*}


\subsection{Reliability Diagram Evaluations}
Put the full reliability diagrams here.

\subsection{Classic Post-hoc Uncertainty Calibration Methods}
\subsubsection{Temperature Scaling}
Temperature scaling is a parametric method that modifies the outputs of a regression model. This modification is controlled by a single parameter, the temperature $T$. The algorithms can be formulated as follows:

\begin{algorithm}[htbp]
\caption{Temperature Scaling for Regression}
\begin{algorithmic}[1]
\STATE Train a model on a training dataset, yielding point predictions $f(x)$.
\STATE Optimize the temperature $T$ on the validation set by minimizing the mean squared error between the predicted and true values.
\FOR{each new input $x$}
\STATE Compute the model's prediction $f(x)$.
\STATE Apply temperature scaling with the learned $T$ to the prediction $f(x)$, yielding scaled prediction $g(f(x))$.
\ENDFOR
\end{algorithmic}
\end{algorithm}

Temperature scaling is an efficient and straightforward method for calibration that requires optimization of only a single parameter. By scaling the outputs, it can yield calibrated predictions without modifying the rank ordering of the model's predictions.

\subsubsection{Isotonic Regression}
Isotonic regression is a non-parametric method utilized for the calibration of a predictive model's outputs. In the context of regression, this method operates as shown below:

\begin{algorithm}[htbp]
\caption{Isotonic Regression for Regression}
\begin{algorithmic}[1]
\STATE Train a model on a training dataset, providing point predictions $f(x)$.
\STATE Fit an isotonic regression model on the validation set predictions $f(x)$, mapping them to calibrated predictions.
\FOR{each new input $x$}
\STATE Compute the model's prediction $f(x)$.
\STATE Use the isotonic regression model to convert the prediction $f(x)$ to a calibrated prediction $g(f(x))$.
\ENDFOR
\end{algorithmic}
\end{algorithm}

Notice that isotonic regression makes no assumptions about the form of the function connecting the model's predictions to calibrated predictions. This flexibility allows it to fit complex, non-linear mappings, which can provide improved calibration performance when the model's outputs are not well-modeled by a simple function.

\subsubsection{Histogram Binning}
Histogram binning can also be applied in a regression setting to calibrate predictions. The idea is to split the range of your model's outputs into several bins, and then adjust the predictions within each bin to match the average actual outcome within that bin. The specific algorithm is:

\begin{algorithm}[htbp]
\caption{Histogram Binning for Regression}
\begin{algorithmic}[1]
\STATE Train a model on a training dataset, yielding predictions $f(x)$.
\STATE Determine the bins for the predictions on the validation set.
\FOR{each bin}
\STATE Compute the average true value for all examples in the bin.
\STATE Adjust the prediction for each example in the bin to the average true value.
\ENDFOR
\FOR{each new input $x$}
\STATE Compute the model's prediction $f(x)$.
\STATE Find the bin that $f(x)$ falls into and adjust $f(x)$ to the average true value for that bin.
\ENDFOR
\end{algorithmic}
\end{algorithm}

This method assumes that predictions within each bin are uniformly mis-calibrated. It is less flexible than isotonic regression, but it is simpler and less prone to overfitting, especially when the number of bins is small.

% \subsubsection{Platt Scaling}
% In a regression setting, Platt Scaling can be interpreted as applying a sigmoid function transformation to the model's outputs. The output is then considered as the mean of a Bernoulli distribution. While this might be useful in some contexts, it is not generally applicable to regression problems because it restricts the outputs to be between 0 and 1. Therefore, Platt scaling might not be suitable for calibration in a general regression setting. \redfont{CITE} has modified the Platt Scaling to make it suitable for the regression task. Therefore, we need to transform the predictions in a way that they are distributed within the range of the target variable. Here is an adapted version of Platt Scaling for regression tasks:

% \subsubsection{Platt Scaling for Regression}
% \begin{algorithm}[htbp]
% \caption{Platt Scaling for Regression}
% \begin{algorithmic}[1]
% \STATE Train a model on a training dataset, yielding predictions $f(x)$.
% \STATE Minimize the mean squared error on the validation set between $g(f(x))$ and the true outcomes, where $g(f(x)) = af(x) + b$ is a linear transformation of the model's predictions.
% \FOR{each new input $x$}
% \STATE Compute the model's prediction $f(x)$.
% \STATE Apply the learned linear transformation to $f(x)$ to get the calibrated prediction.
% \ENDFOR
% \end{algorithmic}
% \end{algorithm}

% In this version of Platt Scaling for regression, a linear transformation is fitted to the model's predictions to minimize the mean squared error on the validation set. The parameters of this transformation are learned from the data, making this an instance of post-hoc calibration. Note that this adaptation might not be suitable for all regression tasks, especially those where the target variable has a non-linear relationship with the features.
